# Supplementary material for: General linear hypothesis testing of high-dimensional mean vectors with unequal covariance matrices based on random integration
Source: arXiv:2410.14120 source file (2024-10-21)
Supplement: Supplementary file 1 [file supplementary_material.pdf]

# Supplementary material for general linear hypothesis testing of high dimensional mean vectors based on random integrals

Mingxiang Cao\* , Yelong Qiu

*Department of Statistics, Anhui Normal University, Wuhu, China*

## 1 The simulation size and power of the other two sample sizes

### 1.1 Simulation results for MANOVA problem

**Table 1** Empirical sizes of  $T_{New}$ ,  $T_Z$ ,  $T_{ZZG}$  and  $T_{ZZ}$  in Case 1.

| n               | p   | $z_{\alpha ik} \stackrel{i.i.d}{\sim} \mathcal{N}(0, 1)$ |        |           |          | $z_{\alpha ik} \stackrel{i.i.d}{\sim} (t_4/\sqrt{2})$ |        |           |          | $z_{\alpha ik} \stackrel{i.i.d}{\sim} (\chi_1^2 - 1)/\sqrt{2}$ |        |           |          |
|-----------------|-----|----------------------------------------------------------|--------|-----------|----------|-------------------------------------------------------|--------|-----------|----------|----------------------------------------------------------------|--------|-----------|----------|
|                 |     | $T_{New}$                                                | $T_Z$  | $T_{ZZG}$ | $T_{ZZ}$ | $T_{New}$                                             | $T_Z$  | $T_{ZZG}$ | $T_{ZZ}$ | $T_{New}$                                                      | $T_Z$  | $T_{ZZG}$ | $T_{ZZ}$ |
| (35,60,80,90)   | 100 | 0.0510                                                   | 0.0560 | 0.0540    | 0.0535   | 0.0510                                                | 0.0595 | 0.0450    | 0.0410   | 0.0520                                                         | 0.0570 | 0.0390    | 0.0385   |
|                 | 200 | 0.0505                                                   | 0.0510 | 0.0490    | 0.0485   | 0.0530                                                | 0.0510 | 0.0380    | 0.0370   | 0.0545                                                         | 0.0565 | 0.0415    | 0.0400   |
|                 | 300 | 0.0520                                                   | 0.0490 | 0.0480    | 0.0475   | 0.0495                                                | 0.0525 | 0.0375    | 0.0365   | 0.0530                                                         | 0.0470 | 0.0375    | 0.0370   |
|                 | 400 | 0.0560                                                   | 0.0540 | 0.0530    | 0.0510   | 0.0530                                                | 0.0550 | 0.0395    | 0.0375   | 0.0555                                                         | 0.0560 | 0.0390    | 0.0385   |
|                 | 500 | 0.0520                                                   | 0.0465 | 0.0460    | 0.0450   | 0.0520                                                | 0.0495 | 0.0360    | 0.0345   | 0.0510                                                         | 0.0525 | 0.0415    | 0.0395   |
| (40,70,100,120) | 100 | 0.0500                                                   | 0.0555 | 0.0520    | 0.0490   | 0.0540                                                | 0.0600 | 0.0435    | 0.0405   | 0.0535                                                         | 0.0530 | 0.0405    | 0.0400   |
|                 | 200 | 0.0510                                                   | 0.0440 | 0.0435    | 0.0425   | 0.0550                                                | 0.0545 | 0.0385    | 0.0375   | 0.0525                                                         | 0.0520 | 0.0410    | 0.0400   |
|                 | 300 | 0.0585                                                   | 0.0580 | 0.0560    | 0.0550   | 0.0525                                                | 0.0530 | 0.0415    | 0.0375   | 0.0490                                                         | 0.0535 | 0.0415    | 0.0395   |
|                 | 400 | 0.0520                                                   | 0.0525 | 0.0515    | 0.0515   | 0.0520                                                | 0.0550 | 0.0430    | 0.0410   | 0.0485                                                         | 0.0505 | 0.0400    | 0.0380   |
|                 | 500 | 0.0530                                                   | 0.0555 | 0.0555    | 0.0535   | 0.0510                                                | 0.0475 | 0.0365    | 0.0350   | 0.0515                                                         | 0.0460 | 0.0340    | 0.0325   |

\*Corresponding author.

E-mail: [caomingx@163.com](mailto:caomingx@163.com)

**Table 2** Empirical sizes of  $T_{New}$ ,  $T_Z$ ,  $T_{ZZG}$  and  $T_{ZZ}$  in Case 2.

| n               | p   | $z_{\alpha ik} \stackrel{i.i.d}{\sim} \mathcal{N}(0, 1)$ |        |           |          | $z_{\alpha ik} \stackrel{i.i.d}{\sim} (t_4/\sqrt{2})$ |        |           |          | $z_{\alpha ik} \stackrel{i.i.d}{\sim} (\chi_1^2 - 1)/\sqrt{2}$ |        |           |          |
|-----------------|-----|----------------------------------------------------------|--------|-----------|----------|-------------------------------------------------------|--------|-----------|----------|----------------------------------------------------------------|--------|-----------|----------|
|                 |     | $T_{New}$                                                | $T_Z$  | $T_{ZZG}$ | $T_{ZZ}$ | $T_{New}$                                             | $T_Z$  | $T_{ZZG}$ | $T_{ZZ}$ | $T_{New}$                                                      | $T_Z$  | $T_{ZZG}$ | $T_{ZZ}$ |
| (35,60,80,90)   | 100 | 0.0550                                                   | 0.0535 | 0.0495    | 0.0490   | 0.0495                                                | 0.0480 | 0.0395    | 0.0370   | 0.0500                                                         | 0.0545 | 0.0470    | 0.0455   |
|                 | 200 | 0.0530                                                   | 0.0540 | 0.0500    | 0.0485   | 0.0500                                                | 0.0525 | 0.0390    | 0.0380   | 0.0520                                                         | 0.0545 | 0.0450    | 0.0425   |
|                 | 300 | 0.0515                                                   | 0.0585 | 0.0565    | 0.0540   | 0.0535                                                | 0.0550 | 0.0455    | 0.0415   | 0.0555                                                         | 0.0525 | 0.0455    | 0.0445   |
|                 | 400 | 0.0525                                                   | 0.0535 | 0.0520    | 0.0510   | 0.0500                                                | 0.0505 | 0.0420    | 0.0395   | 0.0515                                                         | 0.0490 | 0.0415    | 0.0395   |
|                 | 500 | 0.0540                                                   | 0.0460 | 0.0445    | 0.0440   | 0.0515                                                | 0.0545 | 0.0440    | 0.0415   | 0.0500                                                         | 0.0570 | 0.0465    | 0.0450   |
| (40,70,100,120) | 100 | 0.0525                                                   | 0.0455 | 0.0425    | 0.0420   | 0.0525                                                | 0.0570 | 0.0470    | 0.0450   | 0.0515                                                         | 0.0500 | 0.0420    | 0.0410   |
|                 | 200 | 0.0525                                                   | 0.0490 | 0.0470    | 0.0460   | 0.0560                                                | 0.0570 | 0.0505    | 0.0480   | 0.0545                                                         | 0.0530 | 0.0445    | 0.0430   |
|                 | 300 | 0.0530                                                   | 0.0595 | 0.0580    | 0.0550   | 0.0515                                                | 0.0540 | 0.0410    | 0.0400   | 0.0525                                                         | 0.0480 | 0.0400    | 0.0395   |
|                 | 400 | 0.0505                                                   | 0.0560 | 0.0540    | 0.0535   | 0.0490                                                | 0.0520 | 0.0455    | 0.0445   | 0.0540                                                         | 0.0550 | 0.0435    | 0.0425   |
|                 | 500 | 0.0495                                                   | 0.0535 | 0.0510    | 0.0495   | 0.0490                                                | 0.0530 | 0.0420    | 0.0385   | 0.0500                                                         | 0.0525 | 0.0405    | 0.0390   |

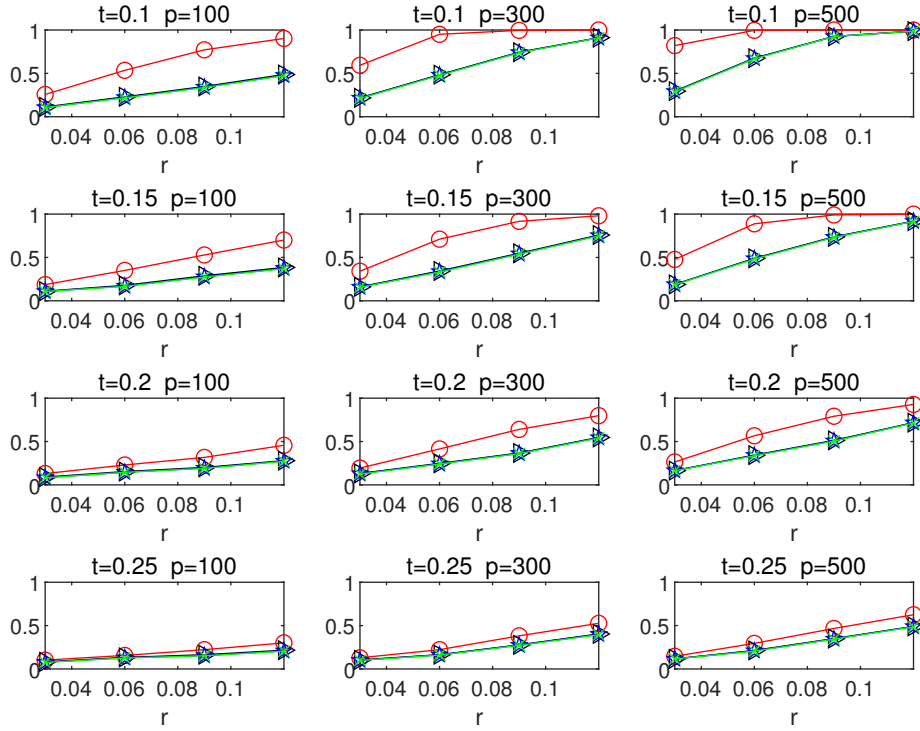

**Figure 1.** For Case 1, under different values of  $r$  and  $t$ , the empirical power of the four tests when  $Z_{\alpha i} \sim \mathcal{N}(0, 1)$ , and  $(n_1, n_2, n_3, n_4) = (35, 60, 80, 90)$ . ( $T_{New}$  : red;  $T_Z$  : black;  $T_{ZZG}$  : blue;  $T_{ZZ}$  : green)

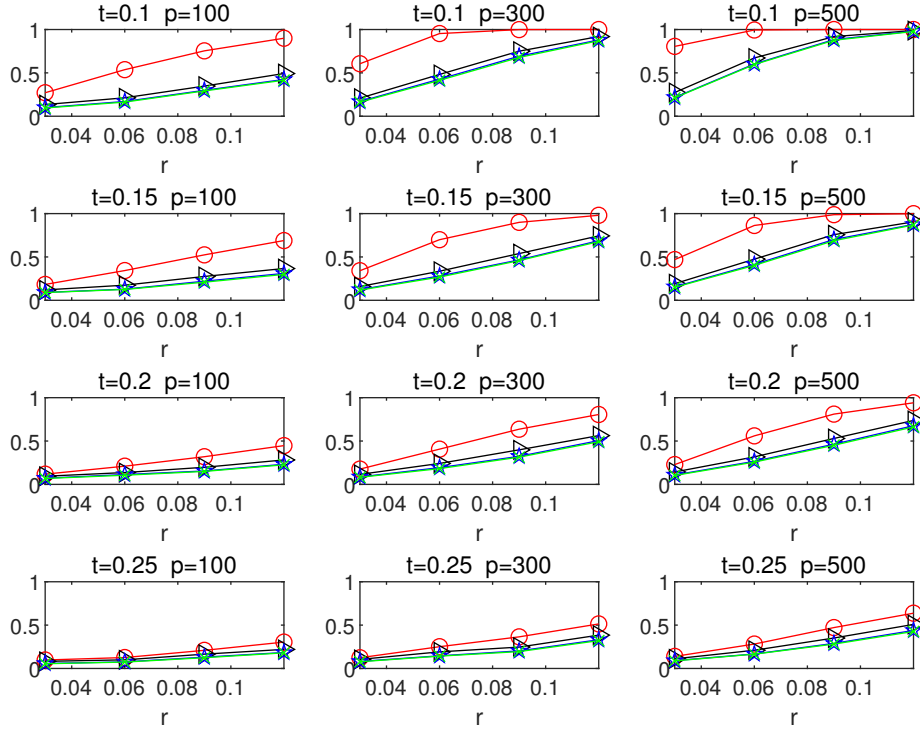

**Figure 2.** For Case 1, under different values of  $r$  and  $t$ , the empirical power of the four tests when  $Z_{\alpha i} \sim t_4/\sqrt{2}$ , and  $(n_1, n_2, n_3, n_4) = (35, 60, 80, 90)$ . ( $T_{New}$  : red;  $T_Z$  : black;  $T_{ZZG}$  : blue;  $T_{ZZ}$  : green)

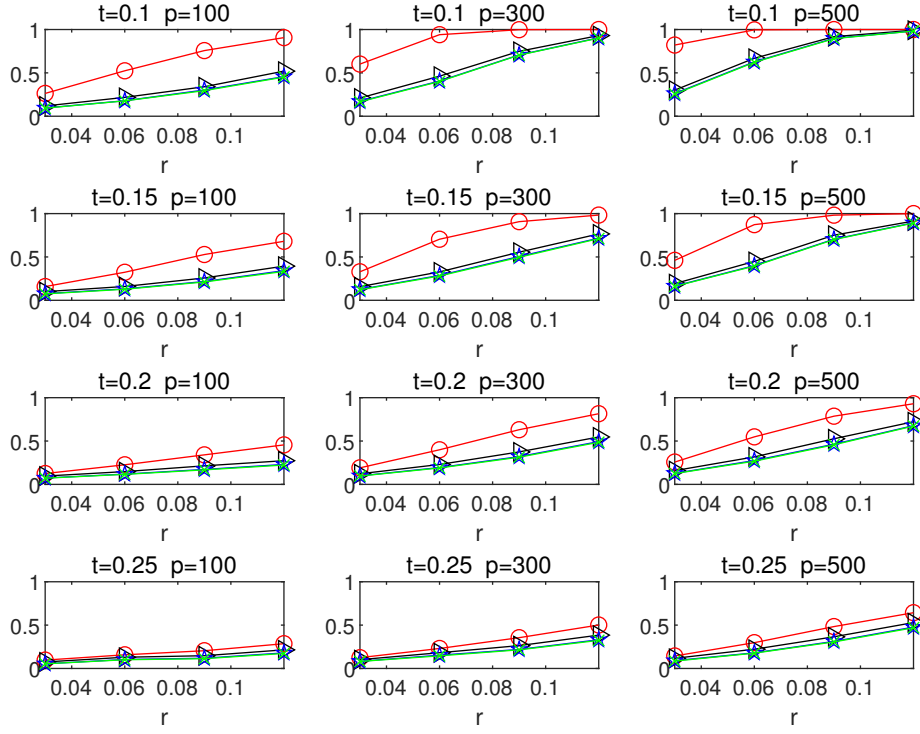

**Figure 3.** For Case 1, under different values of  $r$  and  $t$ , the empirical power of the four tests when  $Z_{\alpha i} \sim (\chi_1^2 - 1)/\sqrt{2}$ , and  $(n_1, n_2, n_3, n_4) = (35, 60, 80, 90)$ . ( $T_{New}$  : red;  $T_Z$  : black;  $T_{ZZG}$  : blue;  $T_{ZZ}$  : green)

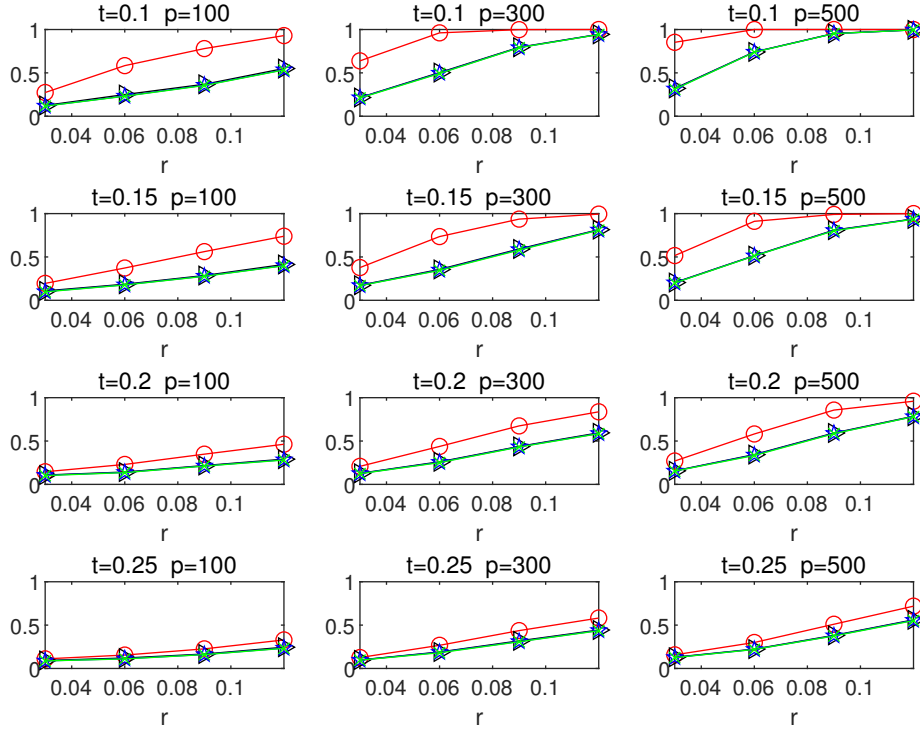

**Figure 4.** For Case 1, under different values of  $r$  and  $t$ , the empirical power of the four tests when  $Z_{\alpha i} \sim N(0, 1)$ , and  $(n_1, n_2, n_3, n_4) = (40, 70, 100, 120)$ . ( $T_{New}$  : red;  $T_Z$  : black;  $T_{ZZG}$  : blue;  $T_{ZZ}$  : green)

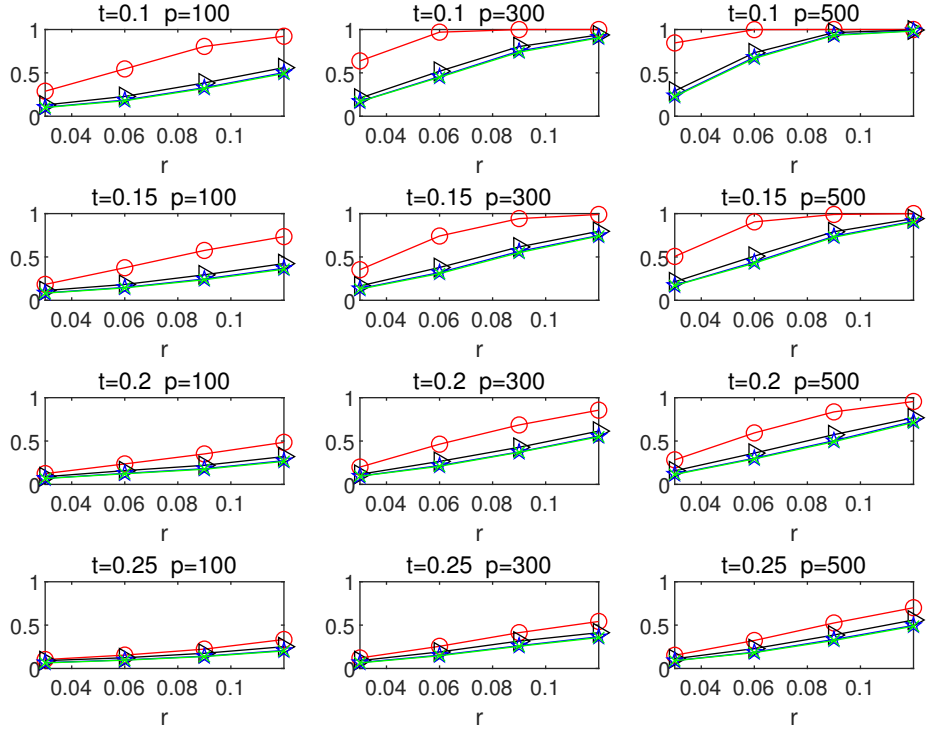

**Figure 5.** For Case 1, under different values of  $r$  and  $t$ , the empirical power of the four tests when  $Z_{\alpha i} \sim t_4/\sqrt{2}$ , and  $(n_1, n_2, n_3, n_4) = (40, 70, 100, 120)$ . ( $T_{New}$  : red;  $T_Z$  : black;  $T_{ZZG}$  : blue;  $T_{ZZ}$  : green)

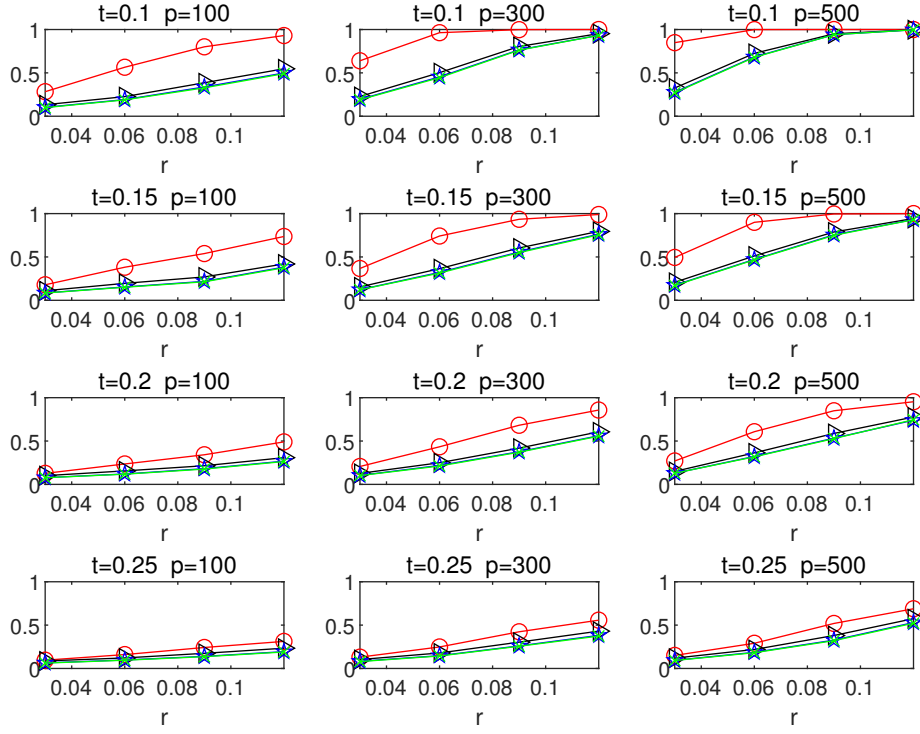

**Figure 6.** For Case 1, under different values of  $r$  and  $t$ , the empirical power of the four tests when  $Z_{\alpha i} \sim (\chi_1^2 - 1)/\sqrt{2}$ , and  $(n_1, n_2, n_3, n_4) = (40, 70, 100, 120)$ . ( $T_{New}$  : red;  $T_Z$  : black;  $T_{ZZG}$  : blue;  $T_{ZZ}$  : green)

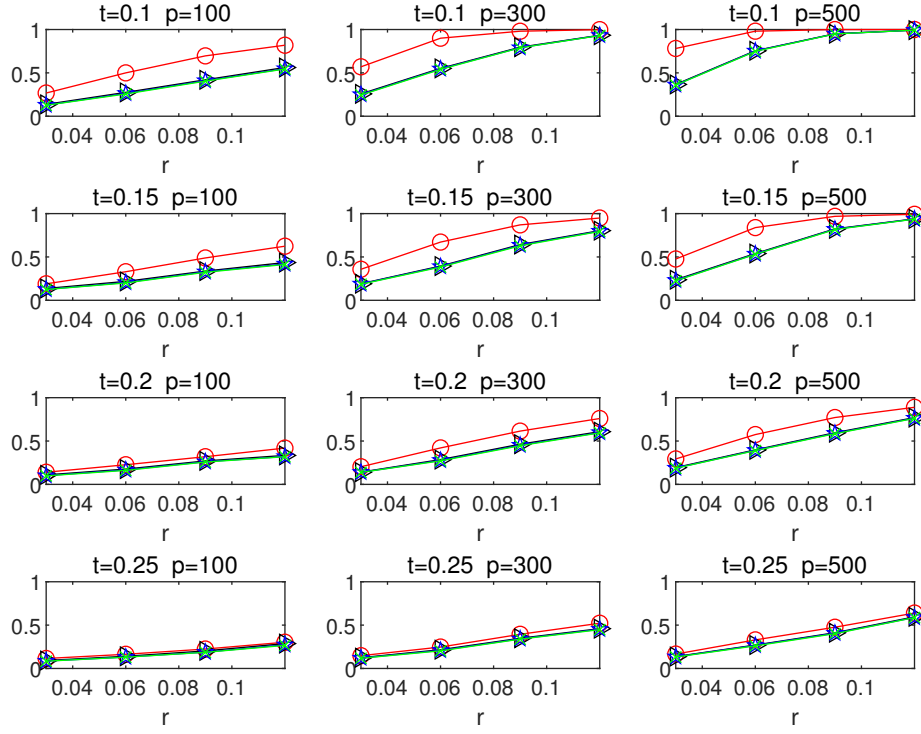

**Figure 7.** For Case 2, under different values of  $r$  and  $t$ , the empirical power of the four tests when  $Z_{\alpha i} \sim N(0, 1)$ , and  $(n_1, n_2, n_3, n_4) = (35, 60, 80, 90)$ . ( $T_{New}$  : red;  $T_Z$  : black;  $T_{ZZG}$  : blue;  $T_{ZZ}$  : green)



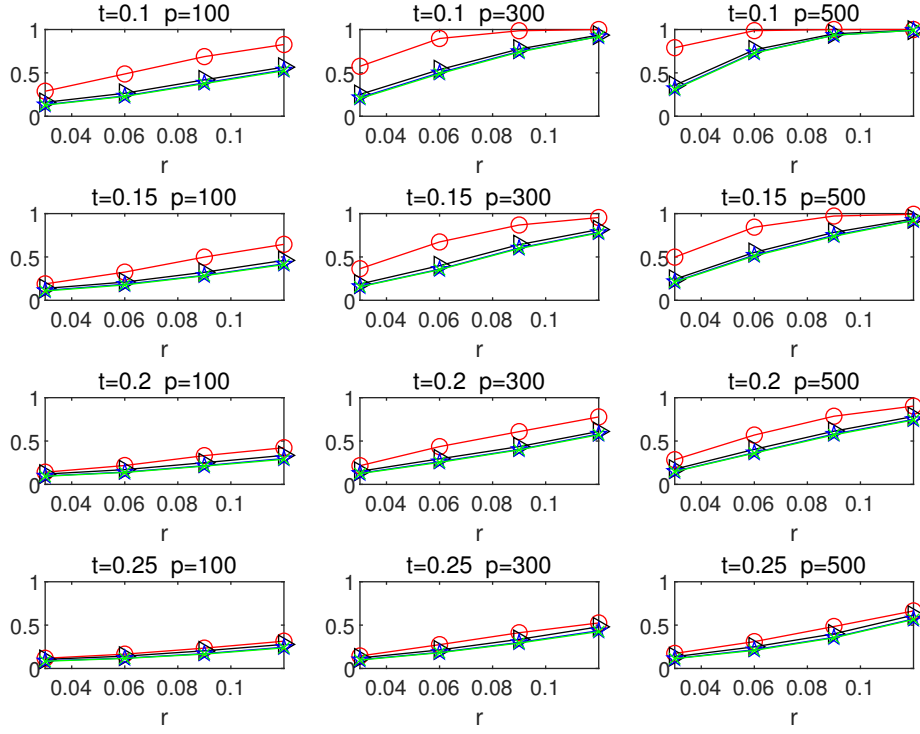

**Figure 8.** For Case 2, under different values of  $r$  and  $t$ , the empirical power of the four tests when  $Z_{\alpha i} \sim t_4/\sqrt{2}$ , and  $(n_1, n_2, n_3, n_4) = (35, 60, 80, 90)$ . ( $T_{New}$  : red;  $T_Z$  : black;  $T_{ZZG}$  : blue;  $T_{ZZ}$  : green)

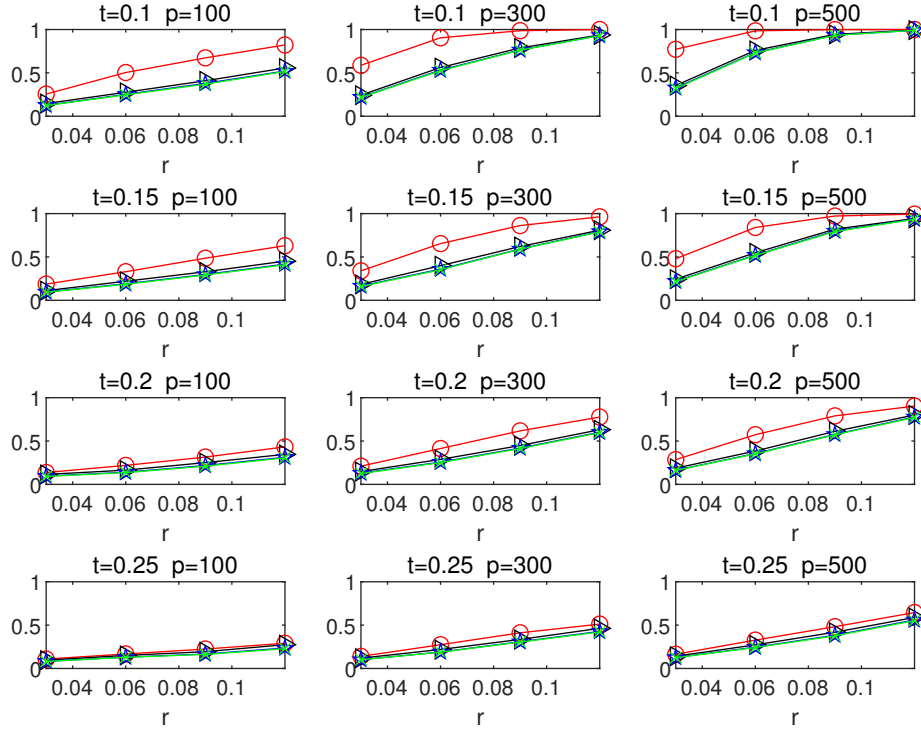

**Figure 9.** For Case 2, under different values of  $r$  and  $t$ , the empirical power of the four tests when  $Z_{\alpha i} \sim (\chi_1^2 - 1)/\sqrt{2}$ , and  $(n_1, n_2, n_3, n_4) = (35, 60, 80, 90)$ . ( $T_{New}$  : red;  $T_Z$  : black;  $T_{ZZG}$  : blue;  $T_{ZZ}$  : green)

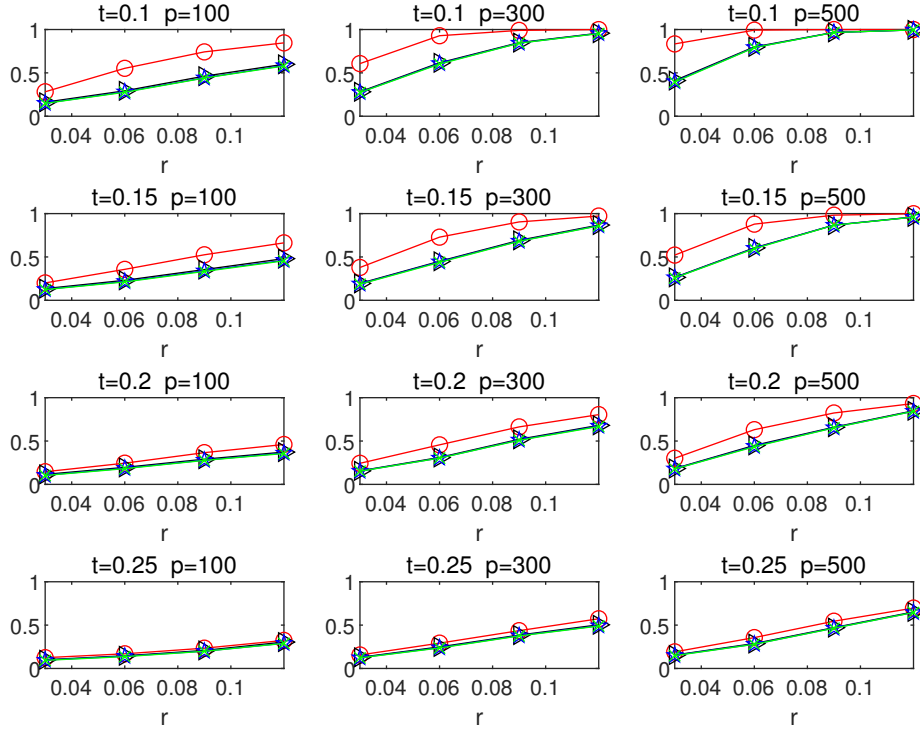

**Figure 10.** For Case 2, under different values of  $r$  and  $t$ , the empirical power of the four tests when  $Z_{\alpha i} \sim N(0, 1)$ , and  $(n_1, n_2, n_3, n_4) = (40, 70, 100, 120)$ . ( $T_{New}$  : red;  $T_Z$  : black;  $T_{ZZG}$  : blue;  $T_{ZZ}$  : green)

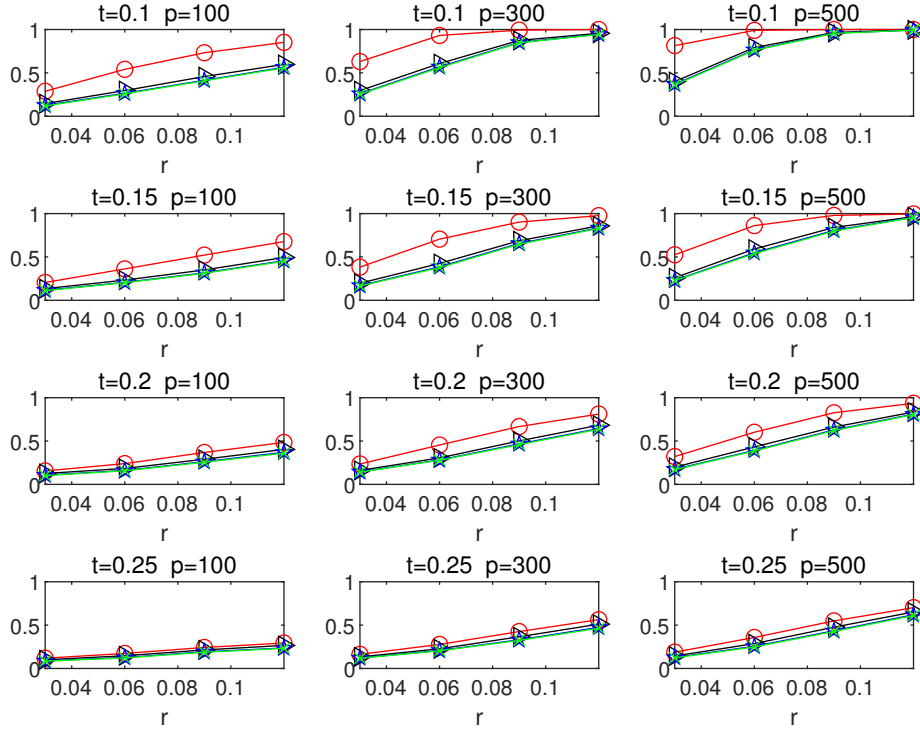

**Figure 11.** For Case 2, under different values of  $r$  and  $t$ , the empirical power of the four tests when  $Z_{\alpha i} \sim t_4/\sqrt{2}$ , and  $(n_1, n_2, n_3, n_4) = (40, 70, 100, 120)$ . ( $T_{New}$  : red;  $T_Z$  : black;  $T_{ZZG}$  : blue;  $T_{ZZ}$  : green)

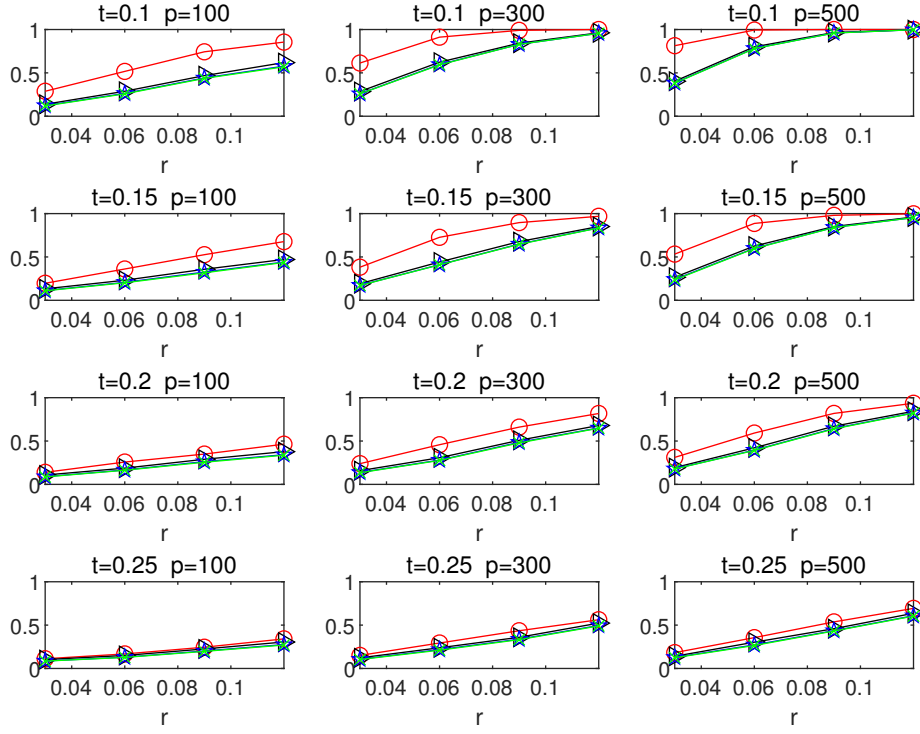

**Figure 12.** For Case 2, under different values of  $r$  and  $t$ , the empirical power of the four tests when  $Z_{\alpha i} \sim (\chi_1^2 - 1)/\sqrt{2}$ , and  $(n_1, n_2, n_3, n_4) = (40, 70, 100, 120)$ . ( $T_{New}$  : red;  $T_Z$  : black;  $T_{ZZG}$  : blue;  $T_{ZZ}$  : green)

## 1.2 Simulation results for GLHT problem

**Table 3** Empirical sizes of  $T_{New}$ ,  $T_Z$ ,  $T_{ZZG}$  and  $T_{ZZ}$  in Case 3.

| n               | p   | $z_{\alpha ik} \stackrel{i.i.d}{\sim} \mathcal{N}(0, 1)$ |        |           |          | $z_{\alpha ik} \stackrel{i.i.d}{\sim} / (t_4/\sqrt{2})$ |        |           |          | $z_{\alpha ik} \stackrel{i.i.d}{\sim} / (\chi_1^2 - 1)/\sqrt{2}$ |        |           |          |
|-----------------|-----|----------------------------------------------------------|--------|-----------|----------|---------------------------------------------------------|--------|-----------|----------|------------------------------------------------------------------|--------|-----------|----------|
|                 |     | $T_{New}$                                                | $T_Z$  | $T_{ZZG}$ | $T_{ZZ}$ | $T_{New}$                                               | $T_Z$  | $T_{ZZG}$ | $T_{ZZ}$ | $T_{New}$                                                        | $T_Z$  | $T_{ZZG}$ | $T_{ZZ}$ |
| (35,60,80,90)   | 100 | 0.0500                                                   | 0.0565 | 0.0485    | 0.0475   | 0.0510                                                  | 0.0560 | 0.0420    | 0.0370   | 0.0540                                                           | 0.0530 | 0.0440    | 0.0425   |
|                 | 200 | 0.0560                                                   | 0.0590 | 0.0560    | 0.0545   | 0.0500                                                  | 0.0460 | 0.0380    | 0.0370   | 0.0540                                                           | 0.0510 | 0.0430    | 0.0410   |
|                 | 300 | 0.0480                                                   | 0.0475 | 0.0425    | 0.0420   | 0.0540                                                  | 0.0545 | 0.0465    | 0.0450   | 0.0535                                                           | 0.0490 | 0.0420    | 0.0420   |
|                 | 400 | 0.0520                                                   | 0.0535 | 0.0485    | 0.0485   | 0.0565                                                  | 0.0455 | 0.0380    | 0.0355   | 0.0490                                                           | 0.0510 | 0.0410    | 0.0395   |
|                 | 500 | 0.0515                                                   | 0.0555 | 0.0490    | 0.0485   | 0.0545                                                  | 0.0510 | 0.0435    | 0.0415   | 0.0530                                                           | 0.0535 | 0.0420    | 0.0405   |
| (40,70,100,120) | 100 | 0.0550                                                   | 0.0455 | 0.0395    | 0.0390   | 0.0540                                                  | 0.0595 | 0.0455    | 0.0445   | 0.0505                                                           | 0.0510 | 0.0390    | 0.0375   |
|                 | 200 | 0.0490                                                   | 0.0485 | 0.0445    | 0.0435   | 0.0530                                                  | 0.0515 | 0.0405    | 0.0385   | 0.0490                                                           | 0.0450 | 0.0370    | 0.0360   |
|                 | 300 | 0.0510                                                   | 0.0510 | 0.0455    | 0.0445   | 0.0540                                                  | 0.0550 | 0.0470    | 0.0460   | 0.0485                                                           | 0.0545 | 0.0435    | 0.0430   |
|                 | 400 | 0.0555                                                   | 0.0560 | 0.0525    | 0.0515   | 0.0510                                                  | 0.0550 | 0.0415    | 0.0400   | 0.0555                                                           | 0.0490 | 0.0430    | 0.0415   |
|                 | 500 | 0.0495                                                   | 0.0465 | 0.0450    | 0.0445   | 0.0500                                                  | 0.0455 | 0.0425    | 0.0420   | 0.0490                                                           | 0.0530 | 0.0455    | 0.0440   |

**Table 4** Empirical sizes of  $T_{New}$ ,  $T_Z$ ,  $T_{ZZG}$  and  $T_{ZZ}$  in Case 4.

| n               | p   | $z_{\alpha ik} \stackrel{i.i.d}{\sim} \mathcal{N}(0, 1)$ |        |           |          | $z_{\alpha ik} \stackrel{i.i.d}{\sim} / (t_4/\sqrt{2})$ |        |           |          | $z_{\alpha ik} \stackrel{i.i.d}{\sim} / (\chi_1^2 - 1)/\sqrt{2}$ |        |           |          |
|-----------------|-----|----------------------------------------------------------|--------|-----------|----------|---------------------------------------------------------|--------|-----------|----------|------------------------------------------------------------------|--------|-----------|----------|
|                 |     | $T_{New}$                                                | $T_Z$  | $T_{ZZG}$ | $T_{ZZ}$ | $T_{New}$                                               | $T_Z$  | $T_{ZZG}$ | $T_{ZZ}$ | $T_{New}$                                                        | $T_Z$  | $T_{ZZG}$ | $T_{ZZ}$ |
| (35,60,80,90)   | 100 | 0.0560                                                   | 0.0645 | 0.0550    | 0.0545   | 0.0540                                                  | 0.0600 | 0.0505    | 0.0500   | 0.0585                                                           | 0.0590 | 0.0470    | 0.0465   |
|                 | 200 | 0.0555                                                   | 0.0655 | 0.0580    | 0.0570   | 0.0575                                                  | 0.0620 | 0.0500    | 0.0490   | 0.0550                                                           | 0.0590 | 0.0515    | 0.0505   |
|                 | 300 | 0.0535                                                   | 0.0525 | 0.0480    | 0.0470   | 0.0515                                                  | 0.0565 | 0.0475    | 0.0465   | 0.0580                                                           | 0.0555 | 0.0475    | 0.0470   |
|                 | 400 | 0.0530                                                   | 0.0540 | 0.0520    | 0.0505   | 0.0550                                                  | 0.0585 | 0.0510    | 0.0505   | 0.0540                                                           | 0.0500 | 0.0445    | 0.0435   |
|                 | 500 | 0.0530                                                   | 0.0605 | 0.0560    | 0.0555   | 0.0580                                                  | 0.0615 | 0.0540    | 0.0530   | 0.0555                                                           | 0.0530 | 0.0460    | 0.0455   |
| (40,70,100,120) | 100 | 0.0565                                                   | 0.0530 | 0.0430    | 0.0425   | 0.0585                                                  | 0.0640 | 0.0510    | 0.0500   | 0.0565                                                           | 0.0560 | 0.0500    | 0.0495   |
|                 | 200 | 0.0520                                                   | 0.0680 | 0.0605    | 0.0600   | 0.0555                                                  | 0.0520 | 0.0470    | 0.0455   | 0.0550                                                           | 0.0580 | 0.0495    | 0.0480   |
|                 | 300 | 0.0510                                                   | 0.0525 | 0.0490    | 0.0480   | 0.0580                                                  | 0.0595 | 0.0485    | 0.0465   | 0.0575                                                           | 0.0455 | 0.0395    | 0.0385   |
|                 | 400 | 0.0530                                                   | 0.0520 | 0.0450    | 0.0445   | 0.0485                                                  | 0.0565 | 0.0495    | 0.0475   | 0.0550                                                           | 0.0510 | 0.0455    | 0.0450   |
|                 | 500 | 0.0490                                                   | 0.0500 | 0.0470    | 0.0465   | 0.0510                                                  | 0.0550 | 0.0470    | 0.0460   | 0.0505                                                           | 0.0520 | 0.0470    | 0.0460   |

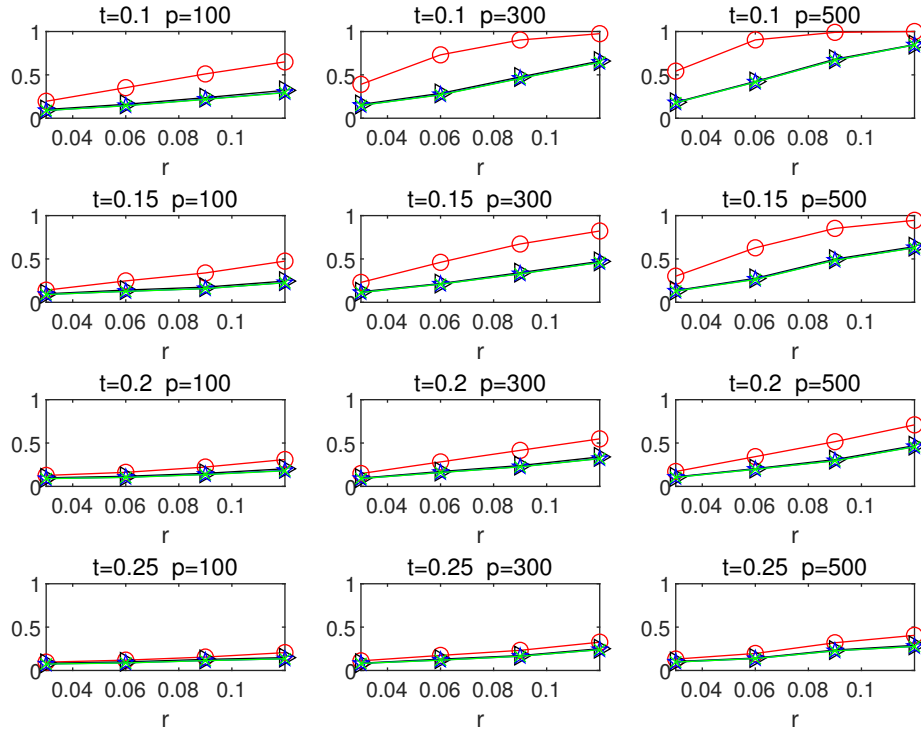

**Figure 13.** For Case 3, under different values of  $r$  and  $t$ , the empirical power of the four tests when  $Z_{\alpha i} \sim N(0, 1)$ , and  $(n_1, n_2, n_3, n_4) = (35, 60, 80, 90)$ . ( $T_{New}$  : red;  $T_Z$  : black;  $T_{ZZG}$  : blue;  $T_{ZZ}$  : green)

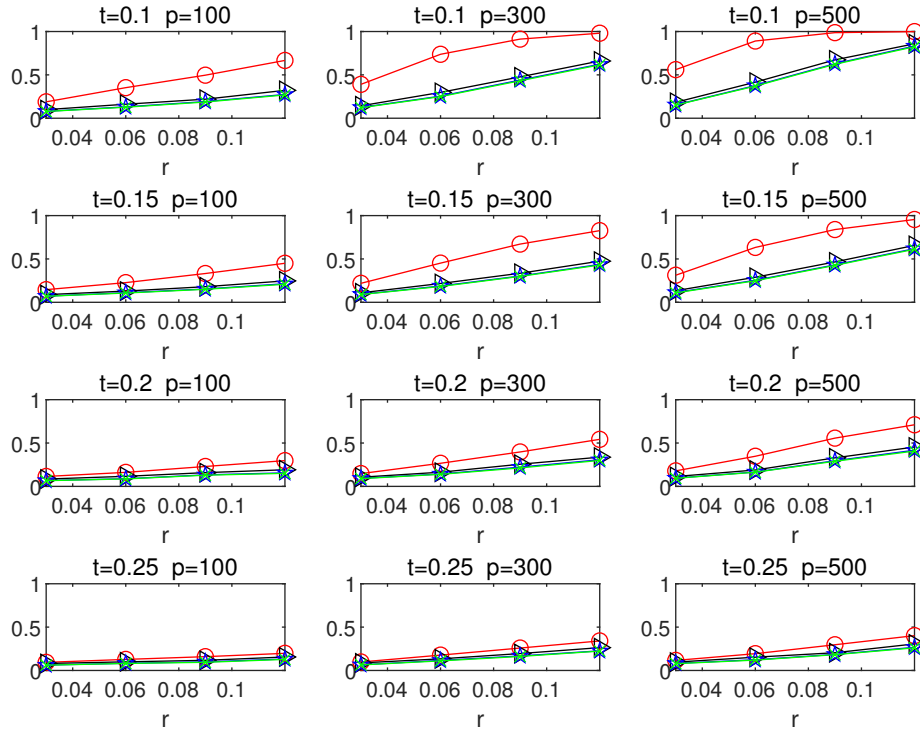

**Figure 14.** For Case 3, under different values of  $r$  and  $t$ , the empirical power of the four tests when  $Z_{\alpha i} \sim t_4/\sqrt{2}$ , and  $(n_1, n_2, n_3, n_4) = (35, 60, 80, 90)$ . ( $T_{New}$  : red;  $T_Z$  : black;  $T_{ZZG}$  : blue;  $T_{ZZ}$  : green)



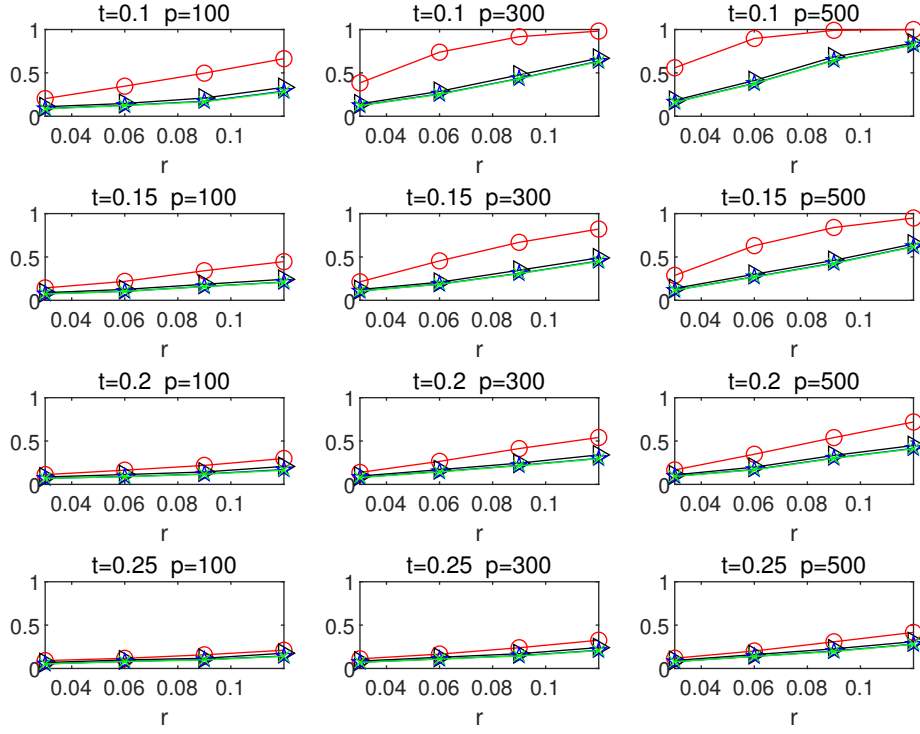

**Figure 15.** For Case 3, under different values of  $r$  and  $t$ , the empirical power of the four tests when  $Z_{\alpha i} \sim (\chi_1^2 - 1)/\sqrt{2}$ , and  $(n_1, n_2, n_3, n_4) = (35, 60, 80, 90)$ . ( $T_{New}$  : red;  $T_Z$  : black;  $T_{ZZG}$  : blue;  $T_{ZZ}$  : green)

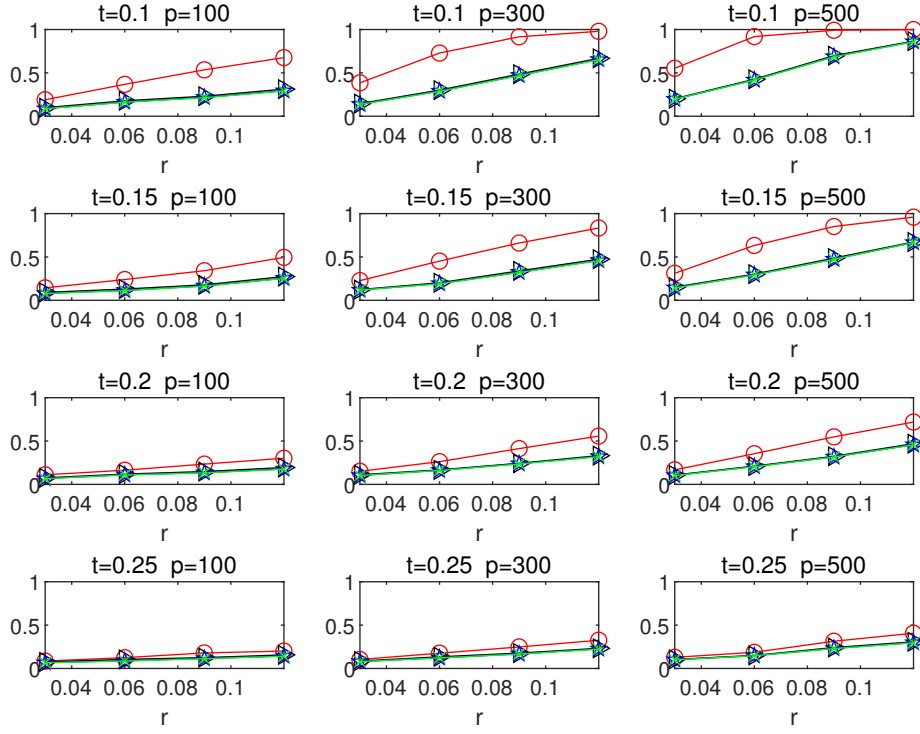

**Figure 16.** For Case 3, under different values of  $r$  and  $t$ , the empirical power of the four tests when  $Z_{\alpha i} \sim N(0, 1)$ , and  $(n_1, n_2, n_3, n_4) = (40, 70, 100, 120)$ . ( $T_{New}$  : red;  $T_Z$  : black;  $T_{ZZG}$  : blue;  $T_{ZZ}$  : green)

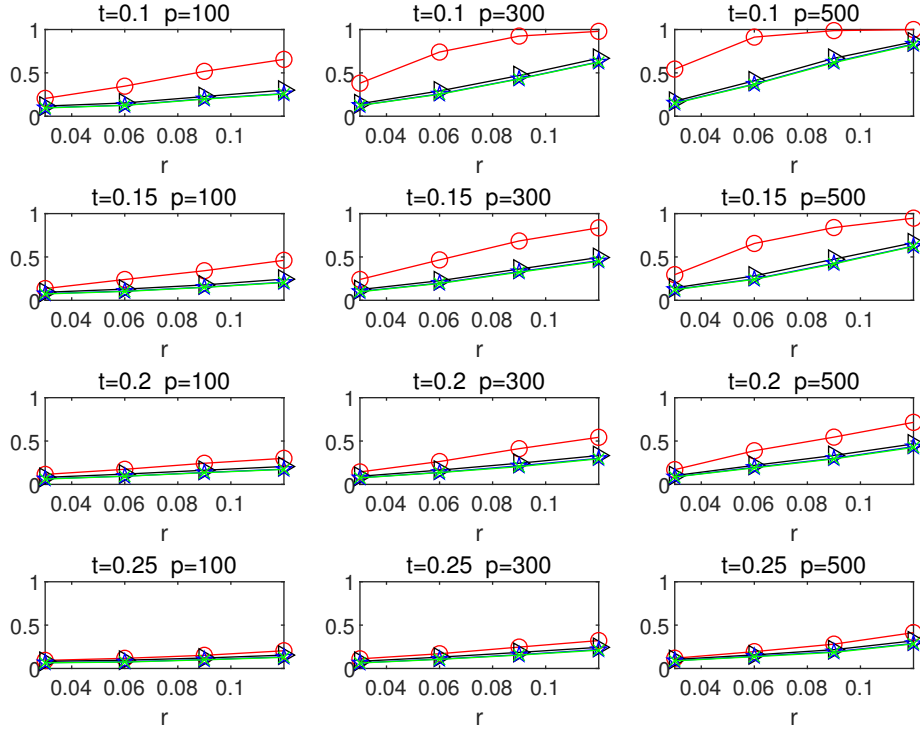

**Figure 17.** For Case 3, under different values of  $r$  and  $t$ , the empirical power of the four tests when  $Z_{\alpha i} \sim t_4/\sqrt{2}$ , and  $(n_1, n_2, n_3, n_4) = (40, 70, 100, 120)$ . ( $T_{New}$  : red;  $T_Z$  : black;  $T_{ZZG}$  : blue;  $T_{ZZ}$  : green)

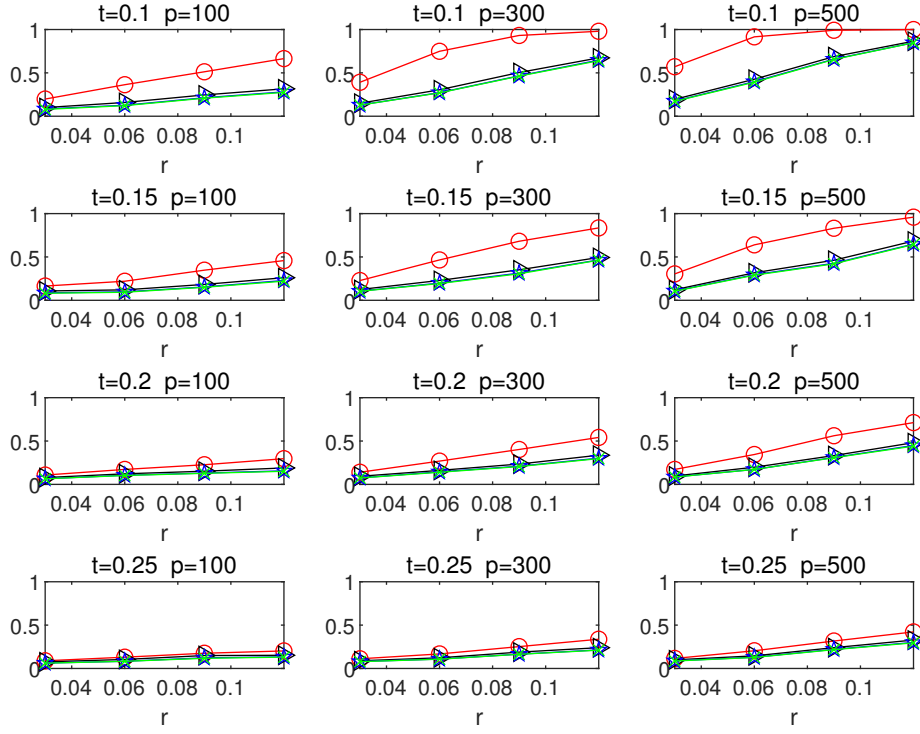

**Figure 18.** For Case 3, under different values of  $r$  and  $t$ , the empirical power of the four tests when  $Z_{\alpha i} \sim (\chi_1^2 - 1)/\sqrt{2}$ , and  $(n_1, n_2, n_3, n_4) = (40, 70, 100, 120)$ . ( $T_{New}$  : red;  $T_Z$  : black;  $T_{ZZG}$  : blue;  $T_{ZZ}$  : green)

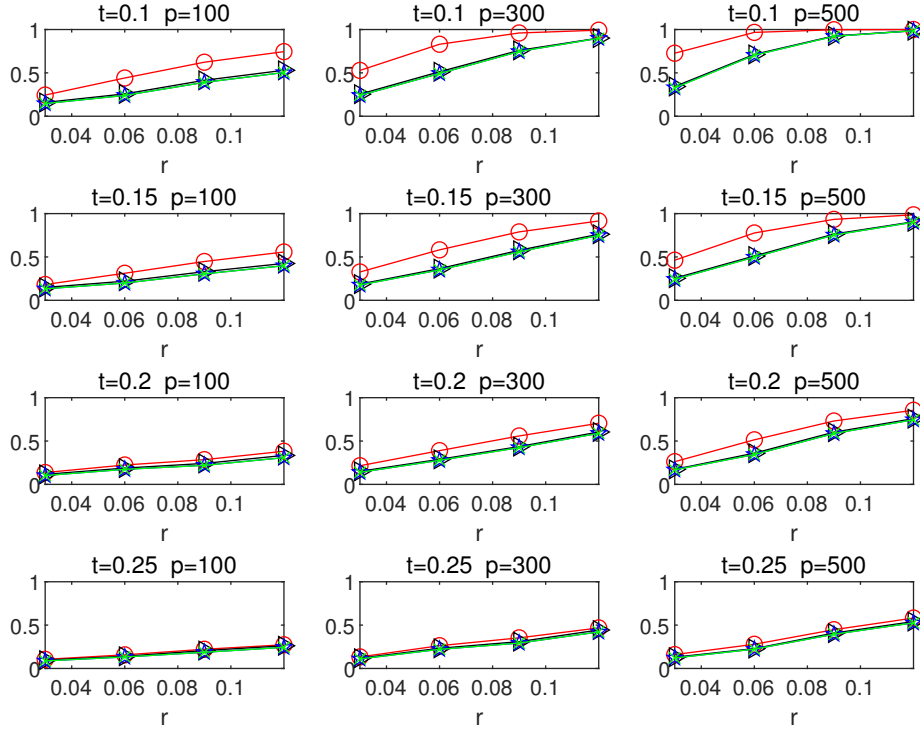

**Figure 19.** For Case 4, under different values of  $r$  and  $t$ , the empirical power of the four tests when  $Z_{\alpha i} \sim N(0, 1)$ , and  $(n_1, n_2, n_3, n_4) = (35, 60, 80, 90)$ . ( $T_{New}$  : red;  $T_Z$  : black;  $T_{ZZG}$  : blue;  $T_{ZZ}$  : green)

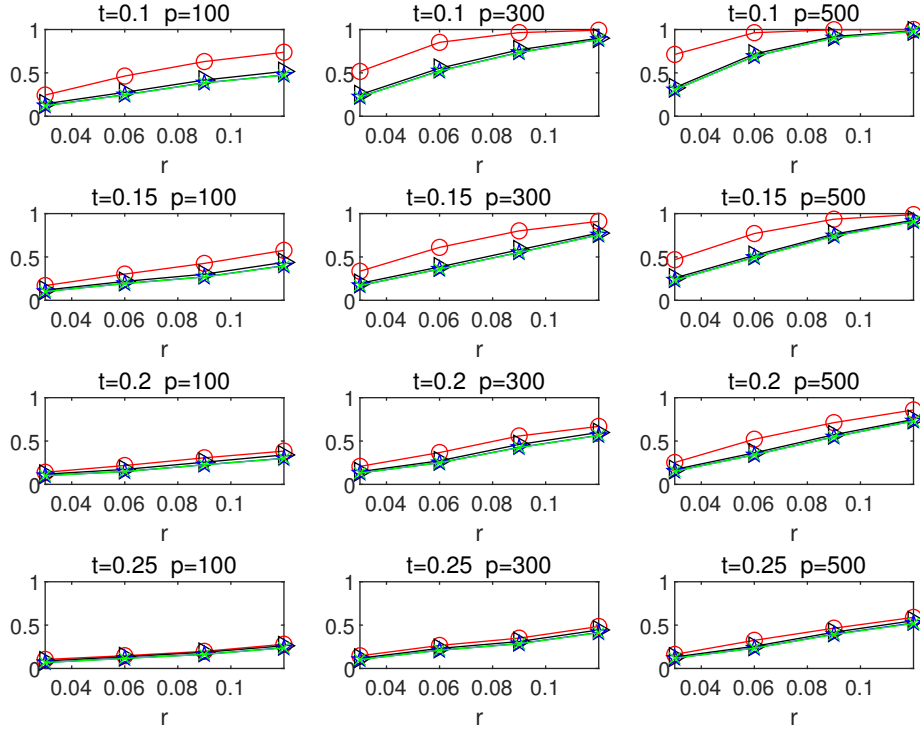

**Figure 20.** For Case 4, under different values of  $r$  and  $t$ , the empirical power of the four tests when  $Z_{\alpha i} \sim t_4/\sqrt{2}$ , and  $(n_1, n_2, n_3, n_4) = (35, 60, 80, 90)$ . ( $T_{New}$  : red;  $T_Z$  : black;  $T_{ZZG}$  : blue;  $T_{ZZ}$  : green)

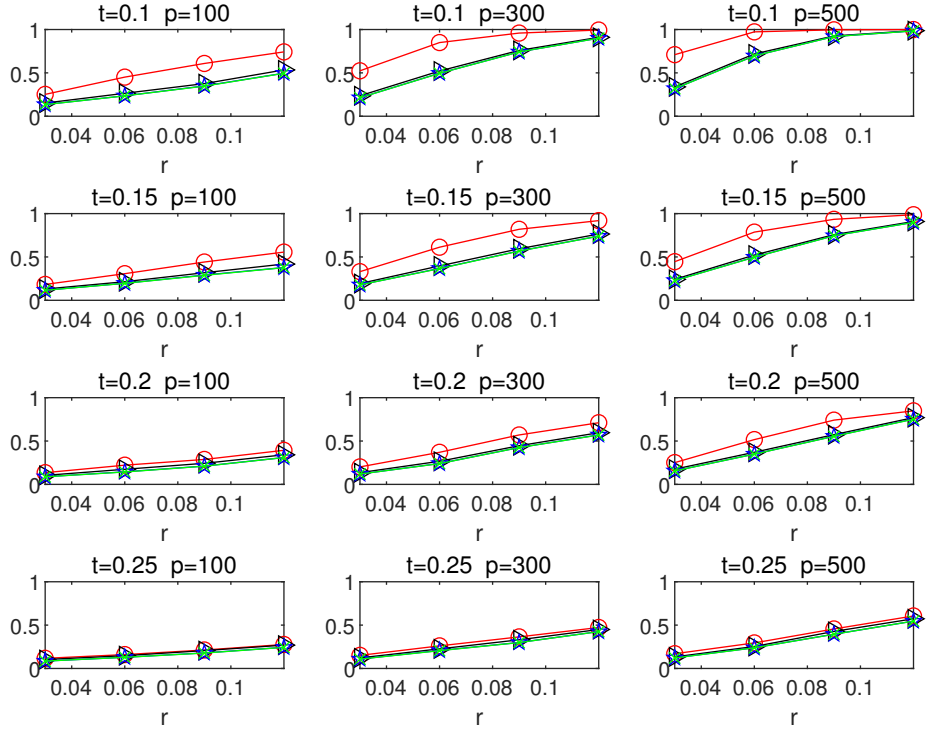

**Figure 21.** For Case 4, under different values of  $r$  and  $t$ , the empirical power of the four tests when  $Z_{\alpha i} \sim (\chi_1^2 - 1)/\sqrt{2}$ , and  $(n_1, n_2, n_3, n_4) = (35, 60, 80, 90)$ . ( $T_{New}$  : red;  $T_Z$  : black;  $T_{ZZG}$  : blue;  $T_{ZZ}$  : green)

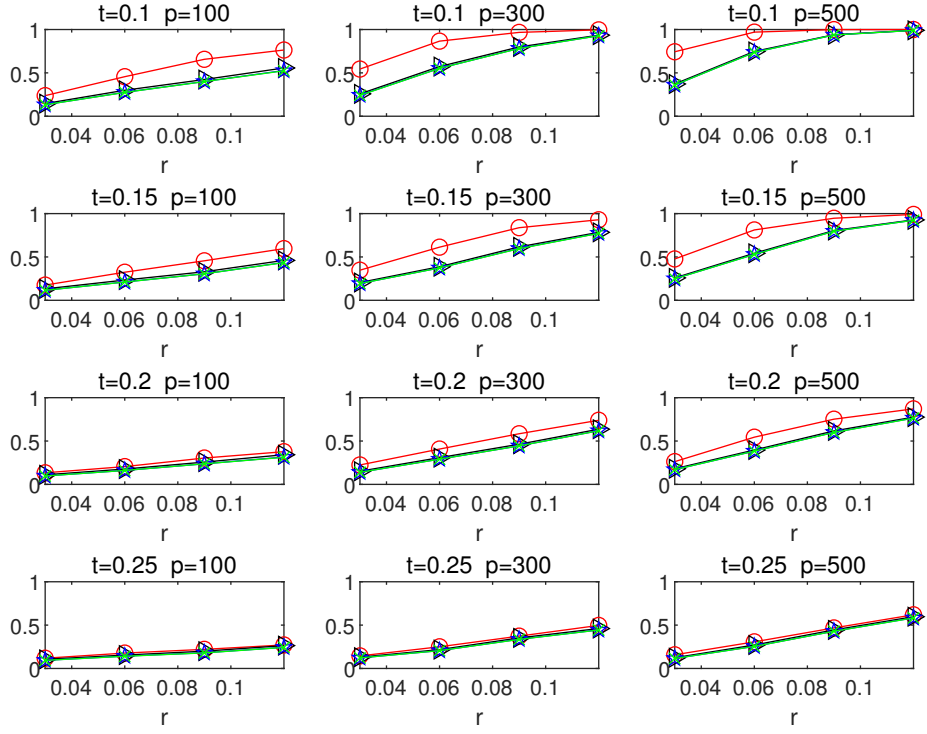

**Figure 22.** For Case 4, under different values of  $r$  and  $t$ , the empirical power of the four tests when  $Z_{\alpha i} \sim N(0, 1)$ , and  $(n_1, n_2, n_3, n_4) = (40, 70, 100, 120)$ . ( $T_{New}$  : red;  $T_Z$  : black;  $T_{ZZG}$  : blue;  $T_{ZZ}$  : green)



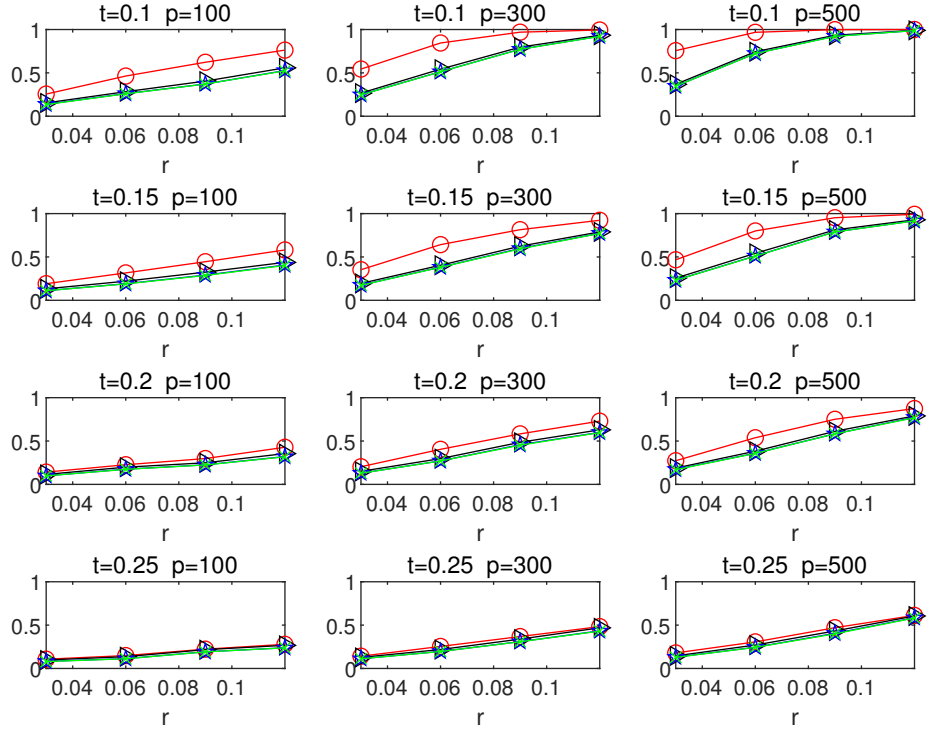

**Figure 23.** For Case 4, under different values of  $r$  and  $t$ , the empirical power of the four tests when  $Z_{\alpha i} \sim t_4/\sqrt{2}$ , and  $(n_1, n_2, n_3, n_4) = (40, 70, 100, 120)$ . ( $T_{New}$  : red;  $T_Z$  : black;  $T_{ZZG}$  : blue;  $T_{ZZ}$  : green)

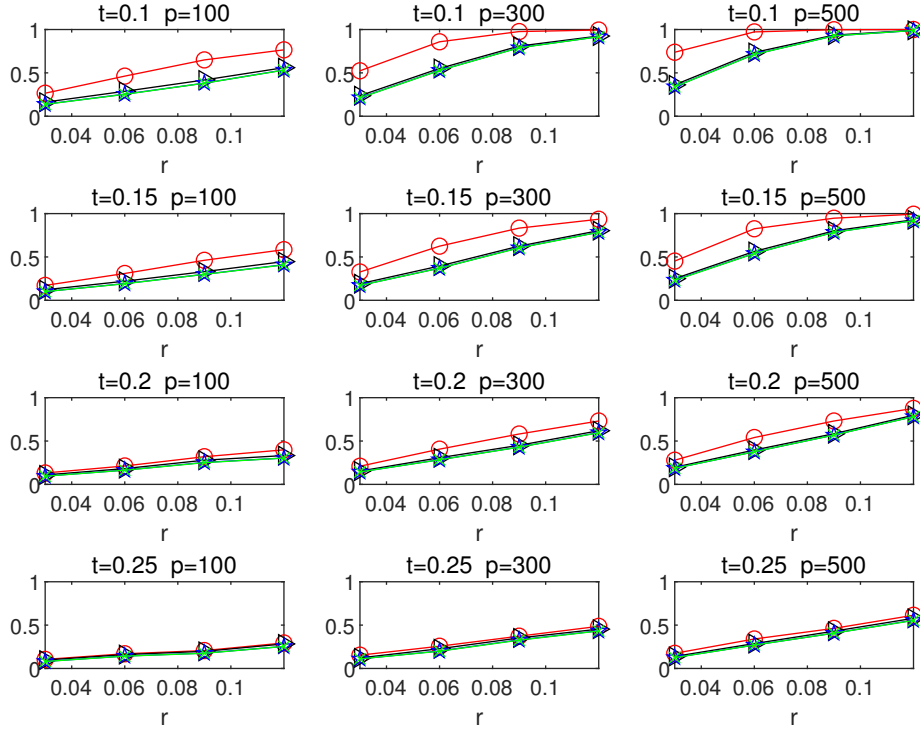

**Figure 24.** For Case 4, under different values of  $r$  and  $t$ , the empirical power of the four tests when  $Z_{\alpha i} \sim (\chi_1^2 - 1)/\sqrt{2}$ , and  $(n_1, n_2, n_3, n_4) = (40, 70, 100, 120)$ . ( $T_{New}$  : red;  $T_Z$  : black;  $T_{ZZG}$  : blue;  $T_{ZZ}$  : green)
